# Supplementary material for: Efficient Predictive Monitoring of Linear Time-Invariant Systems Under Stealthy Attacks
Source: arXiv:2106.02378 source file (2021-06-04)
Supplement: Supplementary file 1 [file section8_appendix.tex]

\section*{Appendix}
%\begingroup
In this appendix, we provide some details regarding the TEP simulation that we used which was originally implemented by Bathelt~\cite{Bathelt_2015_Revision}, and based on the control loops designed by Ricker~\cite{Ricker_Decentralized_1996}.
\begin{itemize}
    \item \textit{Control Inputs (manipulated variables):} \(xmv(1)\) to \(xmv(12)\) as described in~\cite{Downs_plant_1993}, Table 3.
    \item \textit{Controlled Outputs:} \(xmeas(1)\) to \(xmeas(4)\), \(xmeas(7)\) to \(xmeas(12)\), \(xmeas(14)\), \(xmeas(15)\), \(xmeas(17)\), \(xmeas(23)\), \(xmeas(25)\), and \(xmeas(40)\) as described in~\cite{Downs_plant_1993}, Table 4 and Table 5.
\end{itemize}
The safety constraints that we considered for performance evaluations against the number of time steps for prediction and for the illustration of security metrics are given in Table~\ref{table:safety_constraints} (based on Table 6 in~\cite{Downs_plant_1993}).
\begin{table}[h]
\caption{Safety constraints considered for evaluation.}
\label{table:safety_constraints}
    \begin{center}
    \begin{tabular}{ |c|c|c|}
    \hline
    \textbf{Output} & \textbf{Low Limit} & \textbf{High Limit}\\
    \hline
    Reactor Pressure & none & 2895 kPa\\
    \hline
    Reactor Temperature & none & 150 \(\circ C\) \\
    \hline
    Reactor Level & 11.8 \(m^3\) & 21.3 \(m^3\) \\
    \hline
    Product Separator Level & 3.3 \(m^3\) & 9.0 \(m^3\) \\
    \hline
    Stripper Base Level & 3.5 \(m^3\) & 6.6 \(m^3\) \\
    \hline
    \end{tabular}
\end{center}
\end{table}
